# Supplementary material for: Taming False Positives in Out-of-Distribution Detection with Human Feedback
Source: arXiv:2404.16954 source file (2024-04-25)
Supplement: Supplementary file 1 [file iid_case.tex]

We restate the main theorem (Theorem 2) from \cite{howard2022AnytimeValid},
\begin{lemma}
  Let $s_1,\ldots,s_t$ be $i.i.d$ samples drawn from some distribution till time $t$ and let $\hat{F}_t(s) \ldef \frac{1}{t}\sum_{i=1}^t \mathbf{1}\{ s_i \le s\}$ be the empirical CDF at time $t$ and $F_t(s) = \E[\hat{F}_t(s)]$ be the CDF at time $t$. For any $m\ge 1$, $A>1\sqrt{2}$, and $C>0$, the following holds,
  \begin{align*}
    \P \bigg( \exists t\ge m : ||\hat{F}_t - F||_\infty > A \sqrt{\frac{\log \log (et/m) + C }{t}} \bigg ) \le \alpha_{A,C}  \\
   \alpha_{A,C} \ldef \inf_{\eta \in (1,2A^2),  \gamma(A,C,\eta)>1} 4e^{-\gamma^2(A,C,\eta)C}\bigg ( 1 + \frac{1}{(\gamma^2(A,C,\eta)-1) \log \eta}\bigg ) 
  \end{align*}
  where $\gamma(A,C,\eta) \ldef \sqrt{\frac{2}{\eta}}\Big( A- \sqrt{\frac{2(\eta-1)}{C}} \Big )$
\end{lemma}

First, we derive a simplified bound in terms of the failure probability $\delta$ and eliminate other constants.
\begin{lemma}
  Let $s_1,\ldots,s_t$ be $i.i.d$ samples drawn from some distribution till time $t$ and let $\hat{F}_t(s) \ldef \frac{1}{t}\sum_{i=1}^t \mathbf{1}\{ s_i \le s\}$ be the empirical CDF at time $t$ and $F_t(s) = \E[\hat{F}_t(s)]$ be the CDF at time $t$. For any $\delta \in (0,1)$, the following holds,
  \begin{align*}
    \P \bigg( \exists t\ge 1 : ||\hat{F}_t - F||_\infty > \sqrt{\frac{\log \log (et) + \log(100/\delta) }{t}} \bigg ) \le \delta
  \end{align*}
\end{lemma}

\begin{proof}
  Let $A=1,\eta=\frac{9}{8},m=1, C= \frac{c^2}{4}$.
  
  $$\gamma(A,C,\eta) = \sqrt{\frac{2}{\eta}}\Big( A- \sqrt{\frac{2(\eta-1)}{C}} \Big ) = \frac{4}{3}\Big (1-\sqrt{\frac{1}{4C}} \Big ) = \frac{4}{3} \Big(1 - \frac{1}{c} \Big)$$
  
  \begin{align*}
   \alpha_{A,C} &\le 4e^{-\gamma^2(A,C,\eta)C}\bigg ( 1 + \frac{1}{(\gamma^2(A,C,\eta)-1) \log \eta}\bigg )  \\
   &=4\exp \bigg ( - \frac{16}{9} \Big( 1-\frac{1}{c}\Big )^2 \frac{c^2}{4}  \bigg ) \bigg (1 + \frac{1}{ \Big ( \frac{16}{9}\Big(  1-\frac{1}{c} \Big)^2 -1 \Big ) \log 2} \bigg ) \\
   &=4\exp \Big (  -\big( \frac{2}{3}(c-1) \big)^2  \Big ) \Big  (1 + \frac{1}{ \Big ( \frac{16}{9c^2} - \frac{32}{9c} + \frac{7}{9} \Big) \log 2} \bigg ) \\
   &\le 4\exp \Big (  -\big( \frac{2}{3}(c-1) \big)^2  \Big ) \cdot 25 \\
   &= 100 \exp \Big (  -\big( \frac{2}{3}(c-1) \big)^2  \Big ) \\
  \end{align*}
  The last inequality comes by lower bounding $ g(c) =\frac{16}{9c^2} - \frac{32}{9c} + \frac{7}{9}$. First we note that its derivative $g'(c) = \frac{d}{dc}g(c) = \frac{32(c-1)}{9c^3} > 0$ in $(1,\infty)$ hence it is an increasing function in $(1,\infty)$. We restrict ourselves to  $c \ge \sqrt{20}$ giving us $g(c) > 0.07$ for any $c \in (\sqrt{20},\infty)$ and it is easy to see that $1 + \frac{1}{0.07\log(2)} < 25$. Restricting $c \in (\sqrt{20}, \infty) $ means we need to have $C\in [ 5,\infty)$.
  
  Let $\delta =\alpha_{A,C} \le 100\exp( -\big( \frac{2}{3}(c-1) \big)^2 )$ Then for any $\delta \in (0,1)$, solving for $c$ gives the following,
   \begin{align*}
      c &\le \frac{3}{2} \sqrt{\log\frac{100}{\delta}} + 1 \\
       &\le  \frac{3}{2} \sqrt{\log\frac{100}{\delta}} + \frac{1}{2} \sqrt{\log\frac{100}{\delta}}  \\
       &= 2\sqrt{\log\frac{100}{\delta}} \\
   \end{align*}
   This implies $C = \frac{c^2}{4} \le \log(\frac{100}{\delta})$ and for any choice of $\delta \in (0,1)$ we have $C \in [5,\infty)$.
   
\end{proof}

\begin{lemma} (Stopping time)
Let $s_1,\ldots,s_t$ be $i.i.d$ samples drawn from some distribution till time $t$ and let $\hat{F}_t(s) \ldef \frac{1}{t}\sum_{i=1}^t \mathbf{1}\{ s_i \le s\}$ be the empirical CDF at time $t$ and $F_t(s) = \E[\hat{F}_t(s)]$ be the CDF at time $t$. For any $\delta,\alpha \in (0,1)$, the following holds,
  \begin{align*}
    \P \bigg( \exists t\ge T : ||\hat{F}_T - F||_\infty > \alpha \bigg ) \le \delta \quad \text{ for } T = \frac{5}{\alpha^2}\log \Big( \frac{20}{\delta}\log(\frac{10}{\alpha}) \Big)
  \end{align*}
  
\end{lemma}

\begin{proof}
$b_0=100$
$$\psi(t) = \sqrt{\frac{1}{t}\bigg ( \log \Big(\frac{b_0}{\delta} \log(et) \Big )\bigg ) }$$

Let $T = \frac{b_1}{\alpha^2} \log \bigg ( \frac{b_0}{b_3\delta} \log \big ( \frac{b_2}{\alpha} \big )\bigg )$

$\log (x) \le x $ for any $x>0$, and $ \log(ax) \le a \log(x) $ for $x,a>2$.

\begin{align*}
   \psi^2(T)  &= \frac{1}{T} \log \Big [\frac{b_0}{\delta} \log (eT) \Big ] \\
     &= \frac{\alpha^2}{ b_1 \log \Big ( \frac{b_0}{b_3\delta} \log \big ( \frac{b_2}{\alpha} \big )\Big )} \brickred{\log \bigg [ \frac{b_0}{\delta}}  \blue{\log \bigg \{  \frac{e b_1}{\alpha^2} } \green{\log \bigg ( \frac{b_0}{b_3\delta}} \red{ \log \Big ( \frac{b_2}{\alpha} \Big ) }\green{\bigg )} \blue{\bigg \}} \brickred{\bigg ]} \\
   &\overset{\red{a}}{\red{\le}} \frac{\alpha^2}{ b_1 \log \Big ( \frac{b_0}{b_3\delta} \log \big ( \frac{b_2}{\alpha} \big )\Big )}  \brickred{\log \bigg [ \frac{b_0}{\delta}}  \blue{\log \bigg \{  \frac{e b_1}{\alpha^2} } \green{\log \bigg ( \frac{b_0}{b_3\delta}} \red{ \frac{b_2}{\alpha}  }\green{\bigg )} \blue{\bigg \}} \brickred{\bigg ]} \\
   &= \frac{\alpha^2}{ b_1 \log \Big ( \frac{b_0}{b_3\delta} \log \big ( \frac{b_2}{\alpha} \big )\Big )}  \brickred{\log \bigg [ \frac{b_0}{\delta}}  \blue{\log \bigg \{  \frac{e b_1}{\alpha^2} } \green{\log \bigg ( \frac{b_0 b_2}{b_3\delta \alpha} \bigg )} \blue{\bigg \}} \brickred{\bigg ]} \\
   & \green{\overset{b}{\le}} \frac{\alpha^2}{ b_1 \log \Big ( \frac{b_0}{b_3\delta} \log \big ( \frac{b_2}{\alpha} \big )\Big )}  \brickred{\log \bigg [ \frac{b_0}{\delta}}  \blue{\log \bigg \{  \frac{e b_1}{\alpha^2} } \green{  \frac{b_0 b_2}{b_3\delta \alpha} } \blue{\bigg \}} \brickred{\bigg ]} \\
   &=\frac{\alpha^2}{ b_1 \log \Big ( \frac{b_0}{b_3\delta} \log \big ( \frac{b_2}{\alpha} \big )\Big )}  \brickred{\log \bigg [ \frac{b_0}{\delta}}  \blue{\log \bigg \{  \frac{e b_1}{\alpha^2}    \frac{b_0 b_2}{b_3\delta \alpha}  \bigg \}} \brickred{\bigg ]} \\
   &=\frac{\alpha^2}{ b_1 \log \Big ( \frac{b_0}{b_3\delta} \log \big ( \frac{b_2}{\alpha} \big )\Big )} \brickred{\log \bigg [ \frac{b_0}{\delta}}  \blue{\log \bigg \{  \frac{e b_1 b_0 }{b_3 b_2^2 \delta}    \Big ( \frac{b_2}{\alpha} \Big )^3  \bigg \}} \brickred{\bigg ]} \\
   &\overset{\blue{c}}{\blue{\le}}\frac{\alpha^2}{ b_1 \log \Big ( \frac{b_0}{b_3\delta} \log \big ( \frac{b_2}{\alpha} \big )\Big )}  \brickred{\log \bigg [ \frac{b_0}{\delta}}  \blue {\frac{e b_1 b_0 }{b_3  b_2^2 \delta} } \blue{\log \bigg \{   \Big ( \frac{b_2}{\alpha} \Big )^3 \bigg \}   } \brickred{\bigg ]} \\
   &= \frac{\alpha^2}{ b_1 \log \Big ( \frac{b_0}{b_3\delta} \log \big ( \frac{b_2}{\alpha} \big )\Big )}  \brickred{\log \bigg [ \frac{b_0}{\delta}}  \blue {\frac{ 3 e b_1 b_0 }{b_3  b_2^2 \delta} } \blue{\log    \Big ( \frac{b_2}{\alpha} \Big )   } \brickred{\bigg ]} \\
   &=\frac{\alpha^2}{ b_1 \log \Big ( \frac{b_0}{b_3\delta} \log \big ( \frac{b_2}{\alpha} \big )\Big )}  \brickred{\log \bigg [  \Big ( \frac{b_0}{b_3\delta} \Big)^2} \blue{ \frac{3 e b_1 b_3 }{b_2^2} \log    \Big ( \frac{b_2}{\alpha} \Big ) } \brickred{  \bigg ] }\\
   &\blue{\overset{d}{\le}} \frac{\alpha^2 \blue{\frac{3 e b_1 b_3 }{b_2^2}}}{ b_1 \log \Big ( \frac{b_0}{b_3\delta} \log \big ( \frac{b_2}{\alpha} \big )\Big )}  \brickred{\log \bigg [  \Big ( \frac{b_0}{b_3\delta} \Big)^2 } \blue{ \log    \Big ( \frac{b_2}{\alpha} \Big ) } \brickred{  \bigg ] }\\
   & \brickred{\overset{e}{\le}} \frac{ \brickred{2} \alpha^2 \blue{\frac{3 e b_1 b_3 }{b_2^2}}}{ b_1 \log \Big ( \frac{b_0}{b_3\delta} \log \big ( \frac{b_2}{\alpha} \big )\Big )}  \brickred {\log \bigg [   \frac{b_0}{b_3\delta} } \blue{  \log    \Big ( \frac{b_2}{\alpha} \Big ) } \brickred{ \bigg ]} \\
   &=\frac{6\alpha^2 e b_3}{b_2^2}  .
\end{align*}

The inequalities $\brickred{a},\green{b}$ follow from $\log(x)\le x $ for any $x>0$. 

The inequality $\blue{c}$ comes from $\log(ax) \le a \log(x)$ for any $a>2,x>2$. We use $a=\frac{eb_1 b_0}{b_3 b_2^2 \delta}$ and $x=\Big (\frac{b_2}{\alpha} \Big )^3$,
this enforces the following constraints,
 \begin{equation}
 \label{eq:T_up_c1}
     \frac{b_2}{\alpha} > 2^{1/3}
 \end{equation}
 \begin{equation}
 \label{eq:T_up_c2}
     \frac{eb_1 b_0}{b_3 b_2^2 \delta} > 2
 \end{equation}
 For $\blue{d}$ we again use $\log(ax) \le a \log(x)$ with $a=\frac{3eb_1b_3}{b_2^2}$ and $x=  \big ( \frac{b_0}{b_3\delta} \big)^2  \log    \big ( \frac{b_2}{\alpha} \big ) $, this enforces the following constraints,
  \begin{equation}
  \label{eq:T_up_c3}
     \frac{3eb_1b_3}{b_2^2} > 2
 \end{equation}
 \begin{equation}
 \label{eq:T_up_c4}
    \big ( \frac{b_0}{b_3\delta} \big)^2  \log    \big ( \frac{b_2}{\alpha} \big ) > 2
 \end{equation}

 Lastly, $\brickred{e}$ follows by using $\log(x^a y) \le a \log(xy)$ for any $x>0,a>1,y>1$. For this we use $x=\frac{b_0}{b_3\delta}$ and $y=\log(\frac{b_2}{\alpha})$, leading the following constraints,

 \begin{equation}
 \label{eq:T_up_c5}
   \log(\frac{b_2}{\alpha}) > 1
 \end{equation}
 %For $\blue{d}$ and $\brickred{e}$ we use $\log(x^ay) \le a \log(xy)$ for any $a>1,y>1,x>0$. For $\blue{d}$ we use, $a=2$,$x=\frac{b_0}{b_3\delta}$ and $y=$

For $\psi^2(T) \le \alpha^2$, we need 
\begin{equation}
\label{eq:T_up_c6}
   6eb_3 \le b_2^2
\end{equation}

We already have $b_0 =100$, let $b_1=5,b_2=10,b_3 =5$ then the constraints \ref{eq:T_up_c1},\ref{eq:T_up_c2},\ref{eq:T_up_c3},\ref{eq:T_up_c4},\ref{eq:T_up_c5} and \ref{eq:T_up_c6} are satisfied for any $\alpha \in (0,1), \delta \in (0,1)$. Thus we have,

\begin{equation}
  \psi(T) \le \alpha \, \text{ for } T = \frac{5}{\alpha^2}\log \Big( \frac{20}{\delta}\log(\frac{10}{\alpha}) \Big)
\end{equation}

\end{proof}

\subsection{Importance Sampling after $T_0$}
After time point $T_0$, the sampling procedure is modified as follows
\begin{enumerate}
    \item Draw $s_t$ from the original distribution $D$.
    \item If $s_t>\hat{\lambda}_{t-1}$ then observe its true label with probability $p$.
    \item If $s_t\le \hat{\lambda}_{t-1}$ then its label is observed since each point classified as OOD is seen by an expert. 
\end{enumerate}
This modified sampling procedure reduces the labeling burden but introduces two issues, a) the previous estimator of $\FPRhat$ is no longer an unbiased estimator of the true $\FPR$ and b) The samples are not independent anymore due to the dependencies introduced from $\hat{\lambda}_{t-1}$ which depends on previous samples. Due to the presence of dependencies in samples, we can no longer apply the results from \cite{howard2022AnytimeValid} in this regime. 

We address both of these issues by first constructing an unbiased estimator of $\FPRhat$ and then developing novel anytime valid confidence intervals for CDF (cumulative distribution function) estimation with non-independent samples. We observe that the new estimator of $\FPRhat$ is a martingale and thus has an equivalent result of \cite{howard2022AnytimeValid} for martingales will suffice here.

We obtain such results for martingales by extending the results of \cite{balsubramani2015LIL} for CDF estimation.
