# Supplementary material for: Taming False Positives in Out-of-Distribution Detection with Human Feedback
Source: arXiv:2404.16954 source file (2024-04-25)
Supplement: Supplementary file 3 [file cifar-10-knn.tex]

\begin{figure*}[h]
  %\vspace{-8pt}
  \centering
  \includegraphics[width=0.999\textwidth]{figs/fprtpr8/legend.png}
  \mbox{
  \hspace{-10pt}
    \subfigure[No window, no distribution shift.  \label{fig:knn_naive}]{\includegraphics[scale=0.32]{figs/newratio/knn_nowin.png}}
    \hspace{1pt}
    
    \subfigure[10k window, no distribution shift. \label{fig:/knn_win_10k}]{\includegraphics[scale=0.32]{figs/newratio/knn_10kwin.png}}
  }
  \mbox{
  \hspace{-12pt}
    \subfigure[ID:OOD = 2:1 w. distribution shift \& 10k window. \label{fig:knn_shifted_21}]{\includegraphics[scale=0.32]{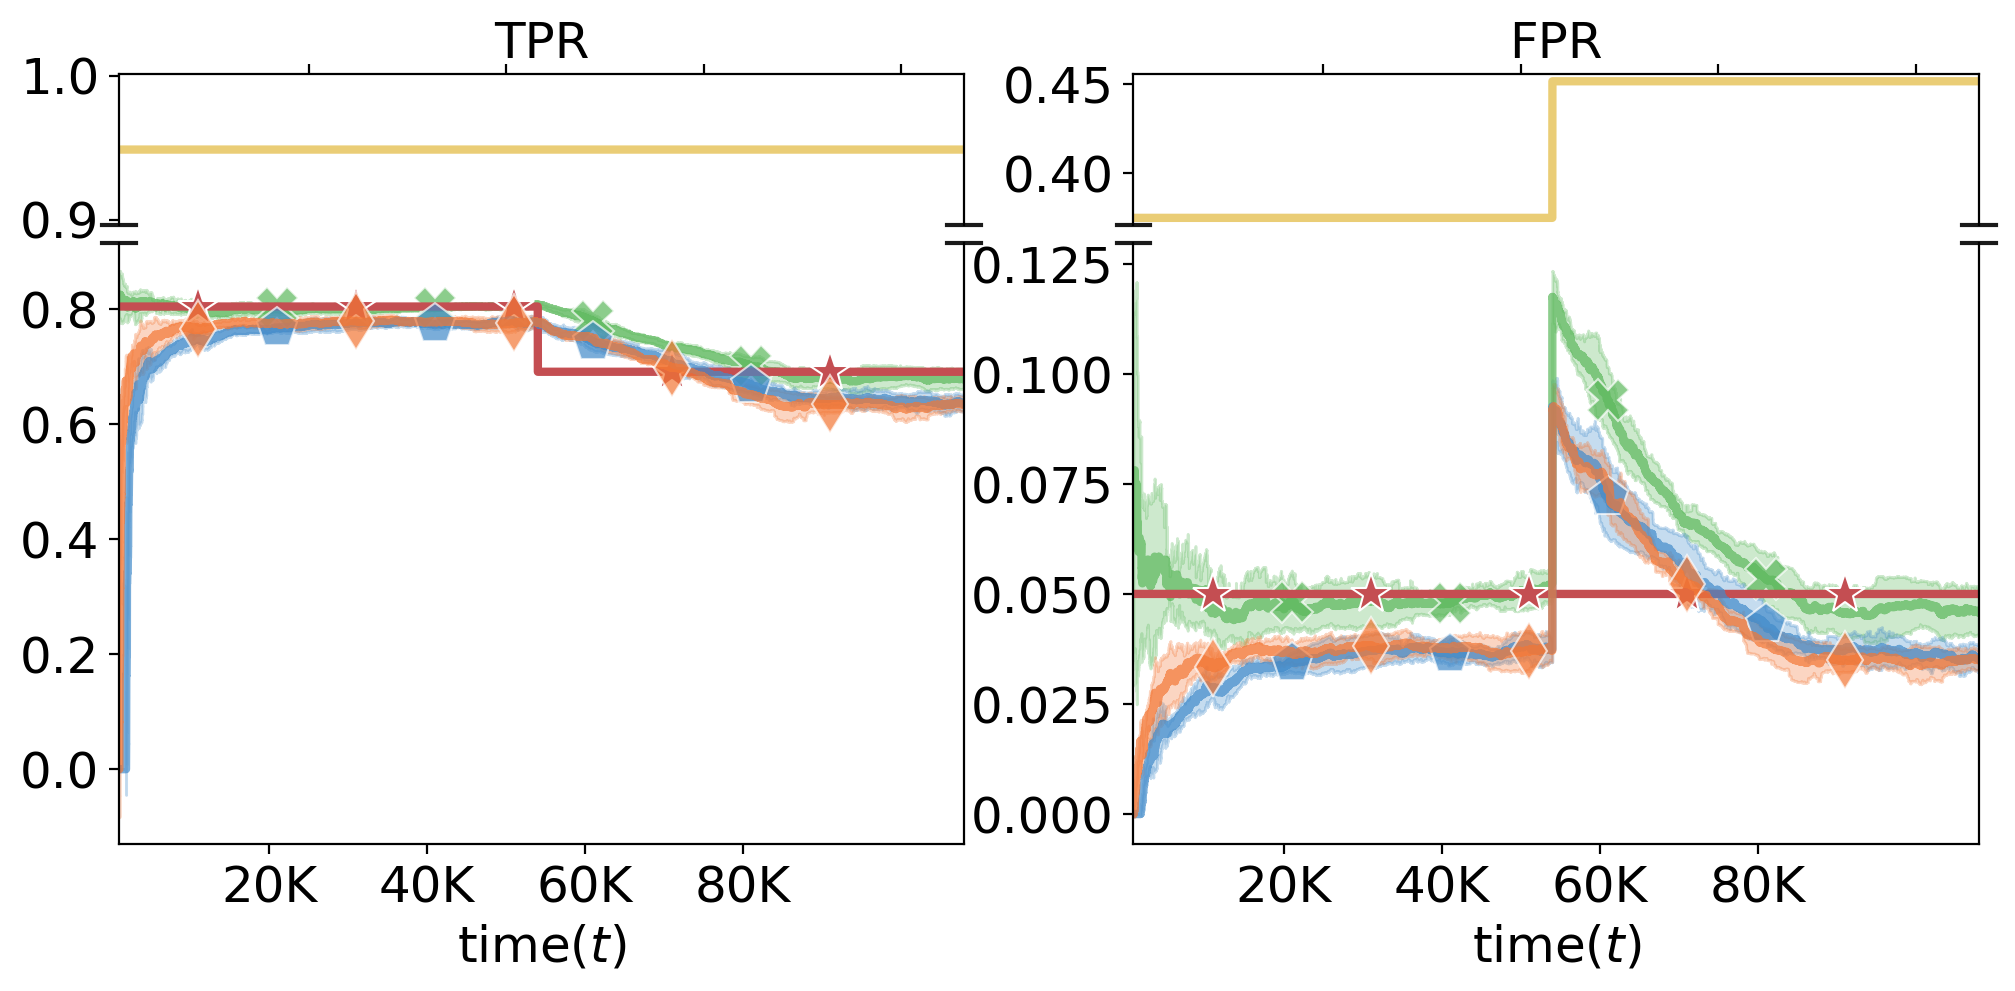}}
    %\hspace{1pt}
    
    \subfigure[ID:OOD = 4:1 w. distribution shift \& 10k window.\label{fig:knn_shifted_41}]{\includegraphics[scale=0.32]{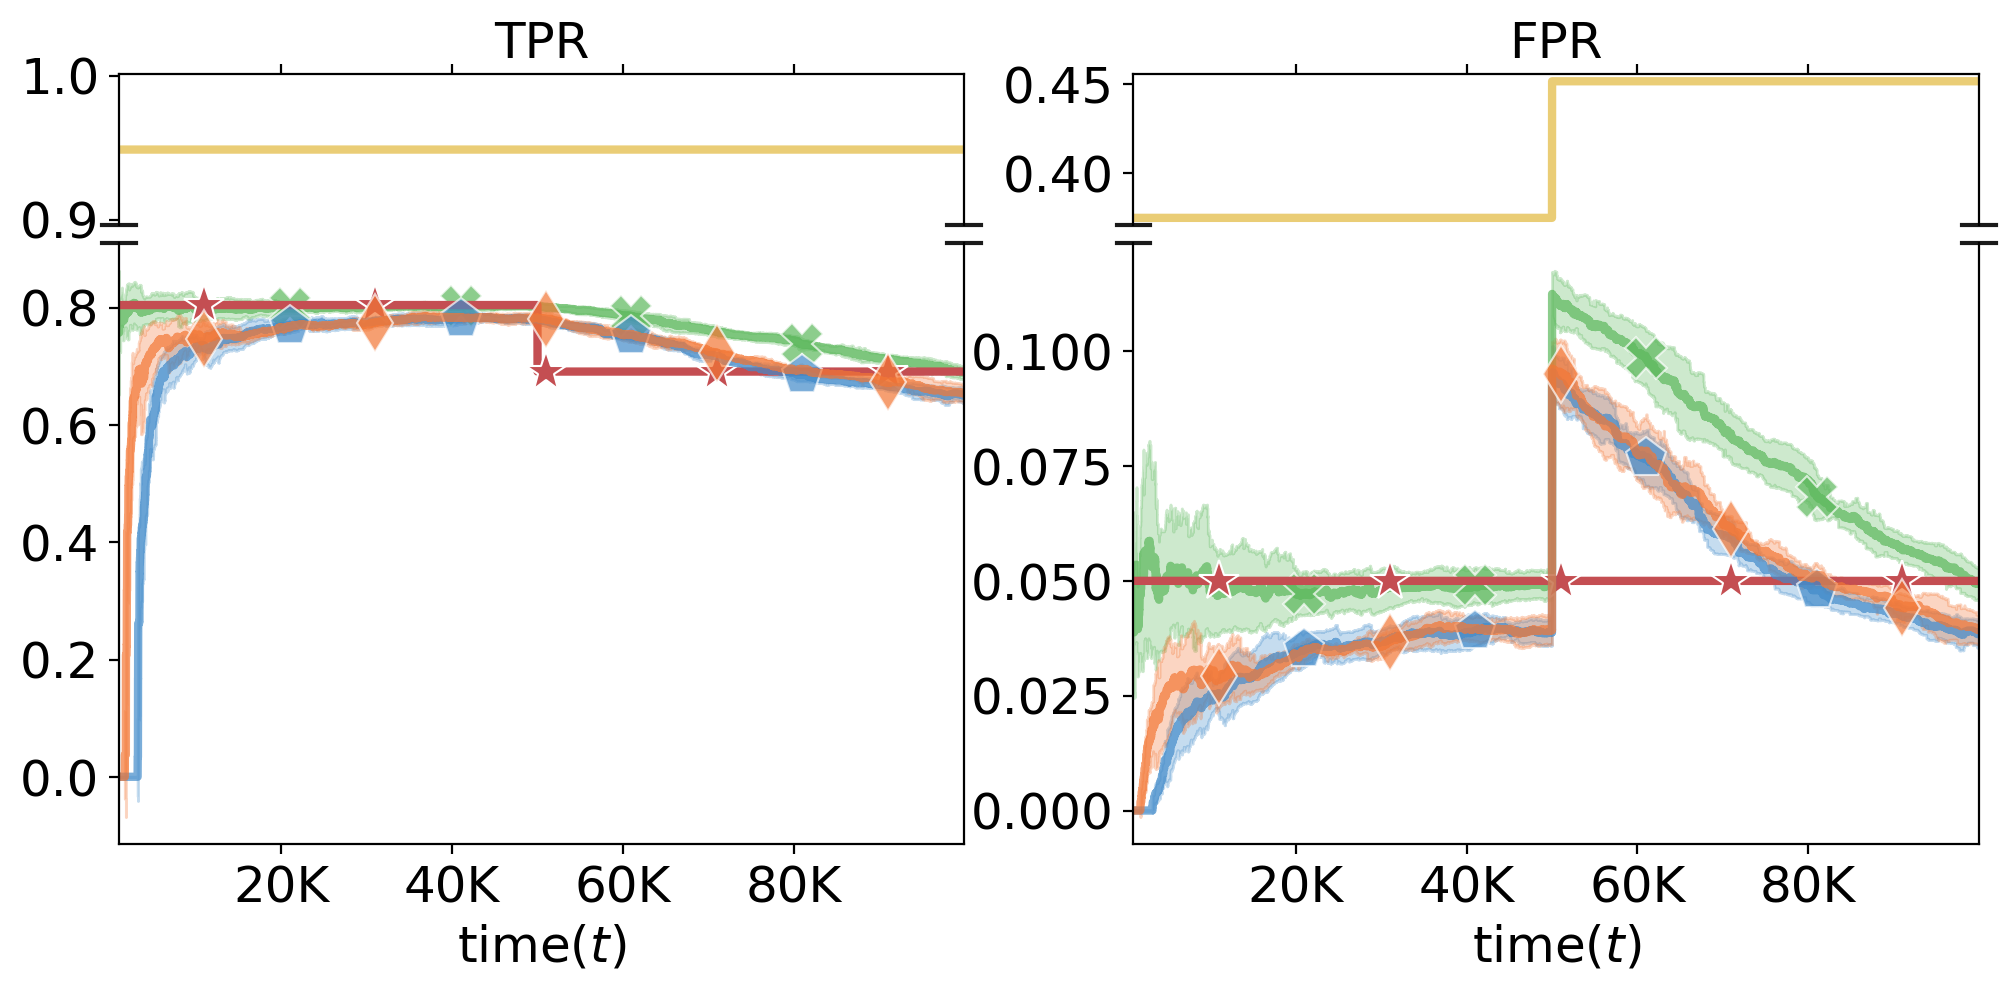}}
  }
  %\vspace{-5pt}
  \caption{
   Results on the KNN scores with Cifar-10 as ID dataset.
    }
  \label{fig:knn-cifar10}
  \vspace{-5pt}
\end{figure*}
