# Supplementary material for: Taming False Positives in Out-of-Distribution Detection with Human Feedback
Source: arXiv:2404.16954 source file (2024-04-25)
Supplement: Supplementary file 4 [file cifar-10-mds.tex]

\begin{figure*}[h]
  \vspace{-8pt}
  \centering
  \includegraphics[width=0.95\textwidth]{figs/fprtpr8/legend.png}
  \mbox{
  \hspace{-10pt}
    \subfigure[No window, no distribution shift.  \label{fig:cifar10_mds}]{\includegraphics[scale=0.17]{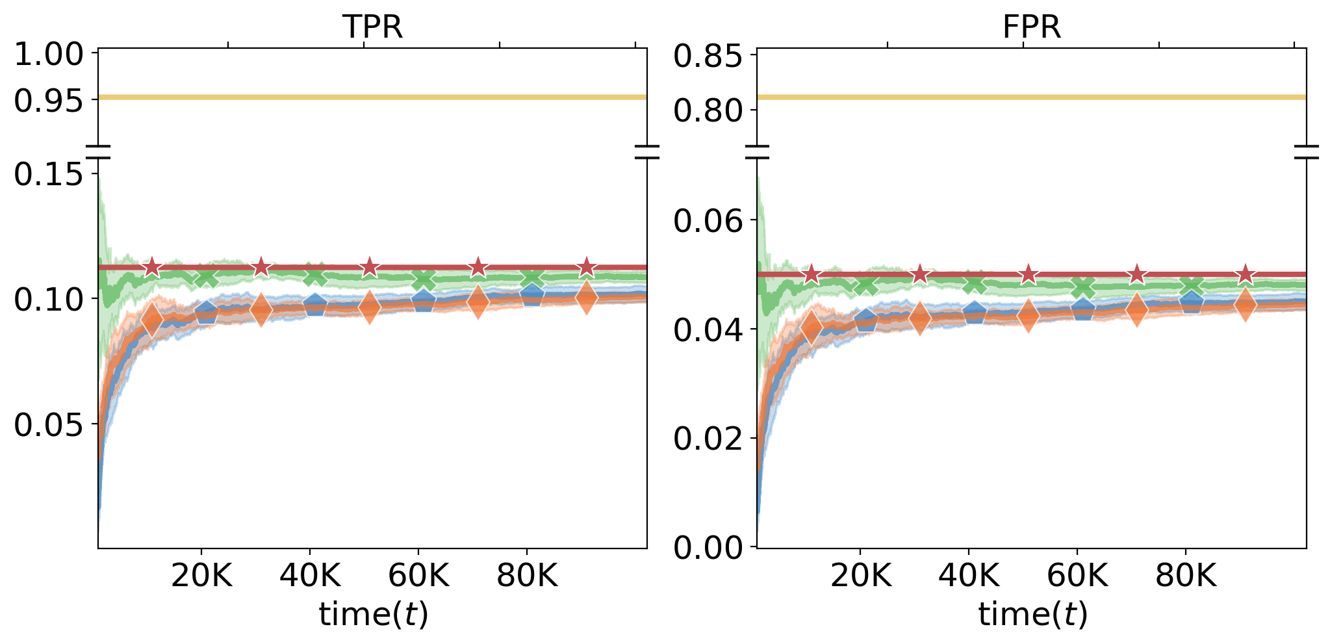}}
    \hspace{1pt}
    
    \subfigure[10k window, no distribution shift. \label{fig:cifar10_mds_win_10}]{\includegraphics[scale=0.17]{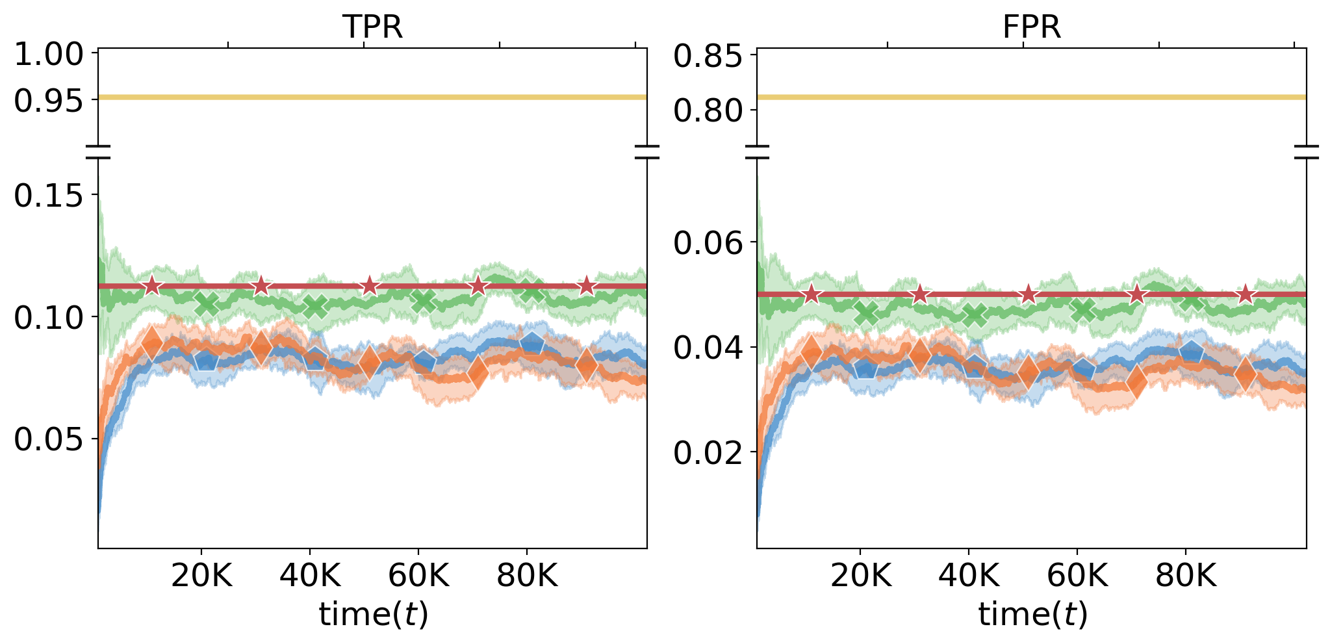}}
  }
  \mbox{
  %\hspace{-10pt}
    \subfigure[No window, distribution shift at $t=45k$. \label{fig:cifar10_mds_shifted}]{\includegraphics[scale=0.17]{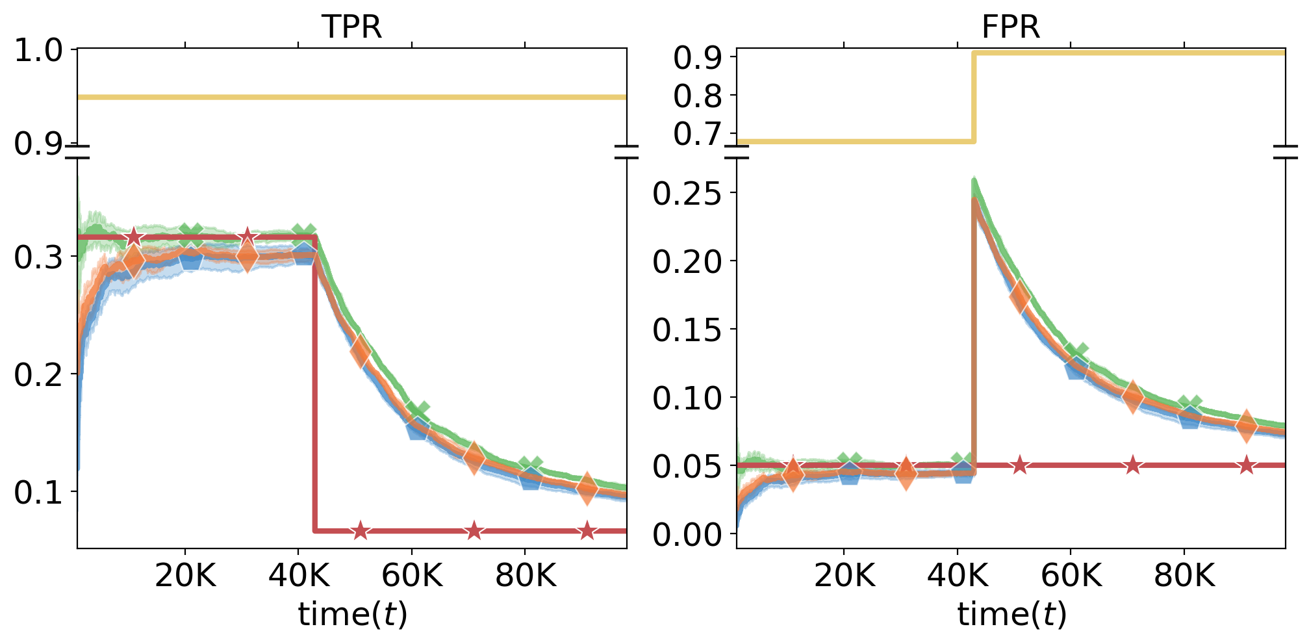}}
    %\hspace{1pt}
    
    \subfigure[10k window, distribution shift at $t=45k$.\label{fig:cifar10_mds_shifted_win_10k}]{\includegraphics[scale=0.17]{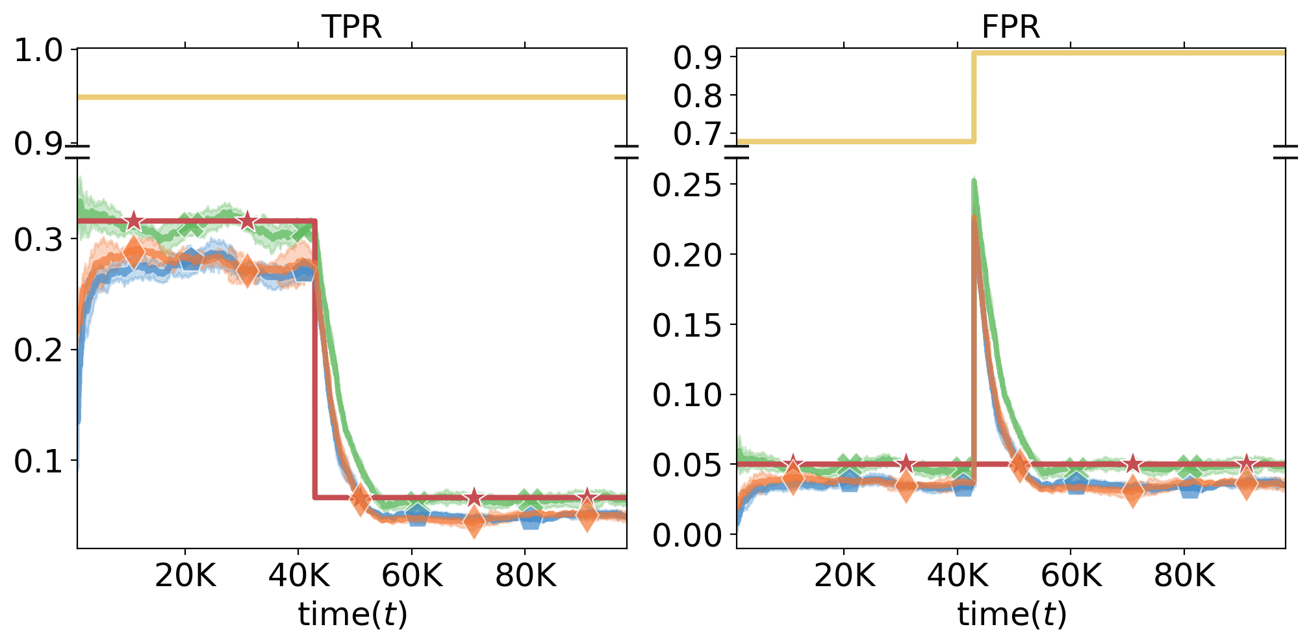}}
  }
  %\vspace{-5pt}
  \caption{
    Results on the Mahalanobis distance (MDS) method with Cifar-10 as the ID dataset. 
    }
  \label{fig:mds-cifar10}
  \vspace{-5pt}
\end{figure*}
