# Supplementary material for: Taming False Positives in Out-of-Distribution Detection with Human Feedback
Source: arXiv:2404.16954 source file (2024-04-25)
Supplement: Supplementary file 7 [file cifar-10-vim.tex]

\begin{figure*}[h]
  \vspace{-8pt}
  \centering
  \includegraphics[width=0.999\textwidth]{figs/fprtpr8/legend.png}
  \mbox{
  \hspace{-10pt}
    \subfigure[No window, no distribution shift.  \label{fig:cifar10_vim}]{\includegraphics[scale=0.16]{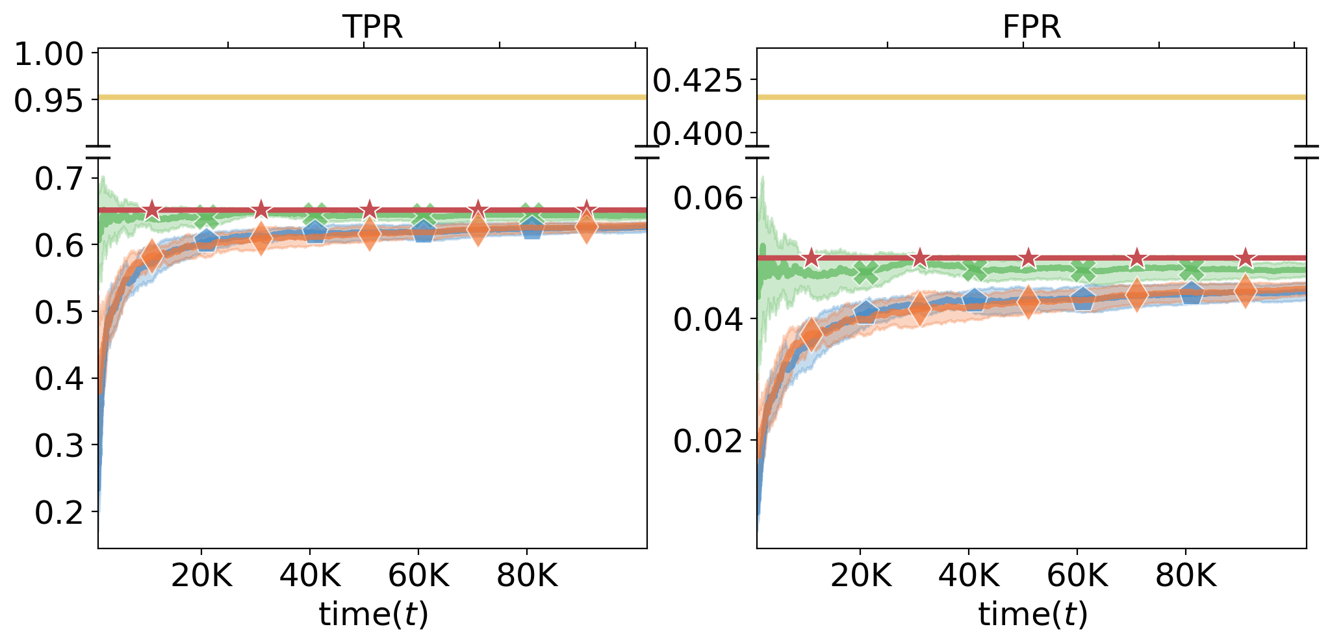}}
    \hspace{1pt}
    
    \subfigure[10k window, no distribution shift. \label{fig:cifar10_vim_win_10}]{\includegraphics[scale=0.16]{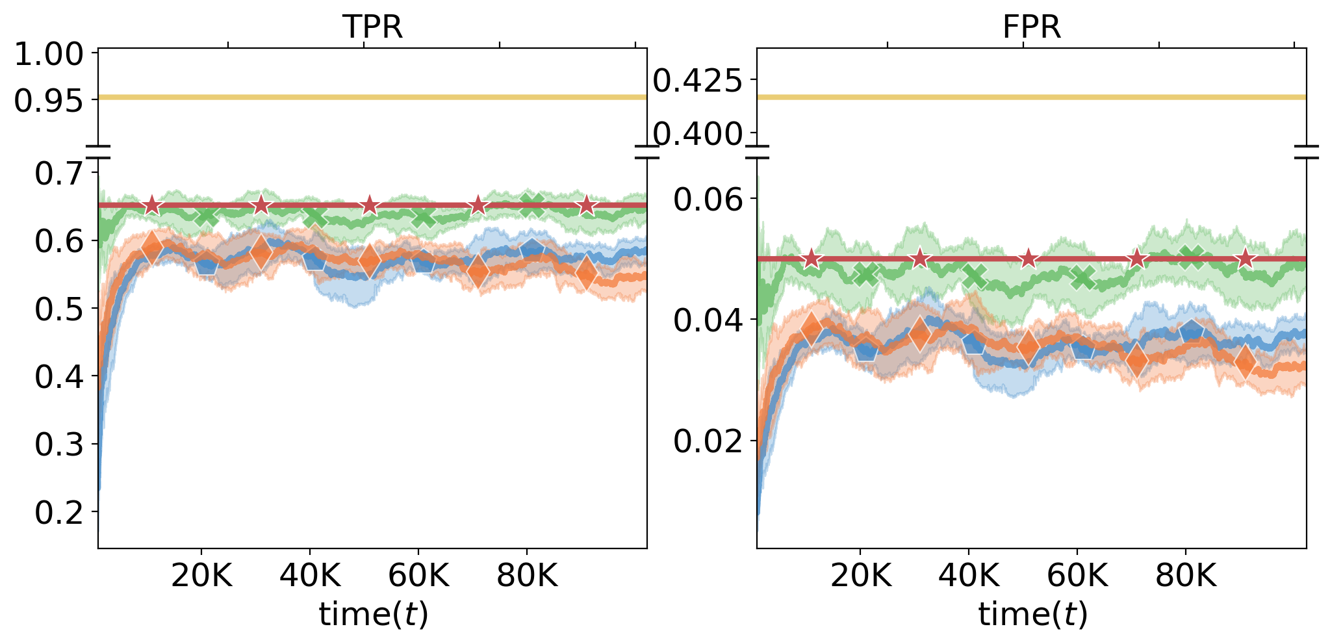}}
  }
  \mbox{
  \hspace{-12pt}
    \subfigure[No window, distribution shift at $t=45k$. \label{fig:cifar10_vim_shifted}]{\includegraphics[scale=0.16]{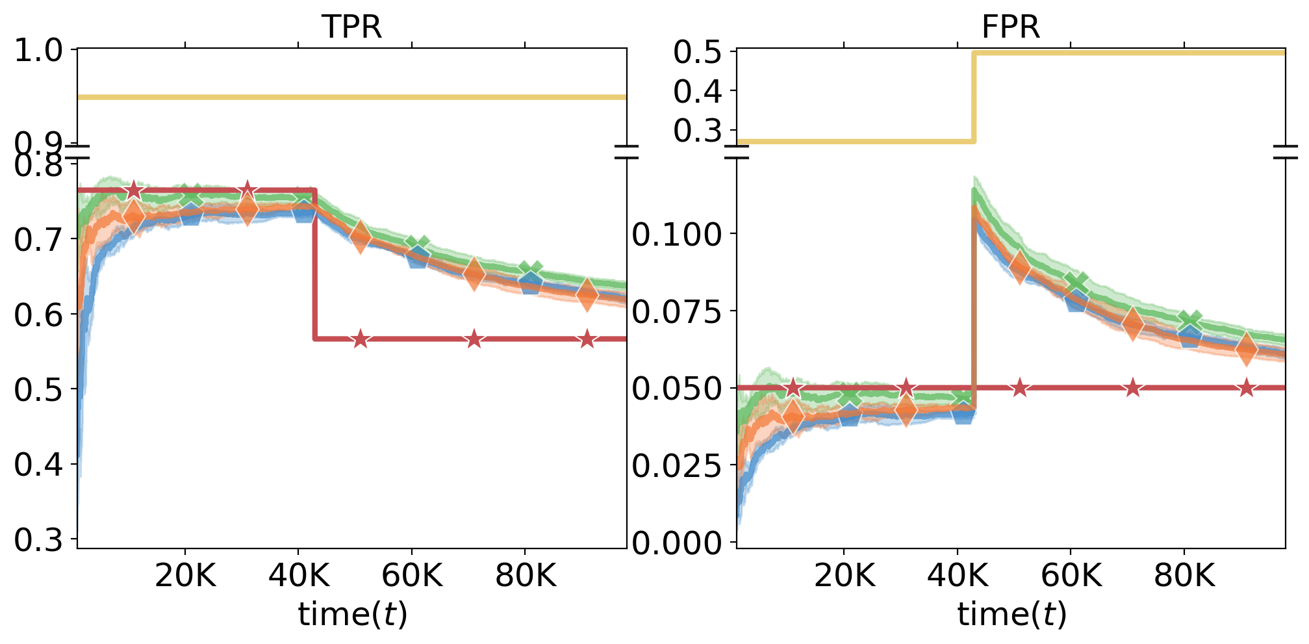}}
    %\hspace{1pt}
    
    \subfigure[10k window, distribution shift at $t=45k$.\label{fig:cifar10_vim_shifted_win_10k}]{\includegraphics[scale=0.17]{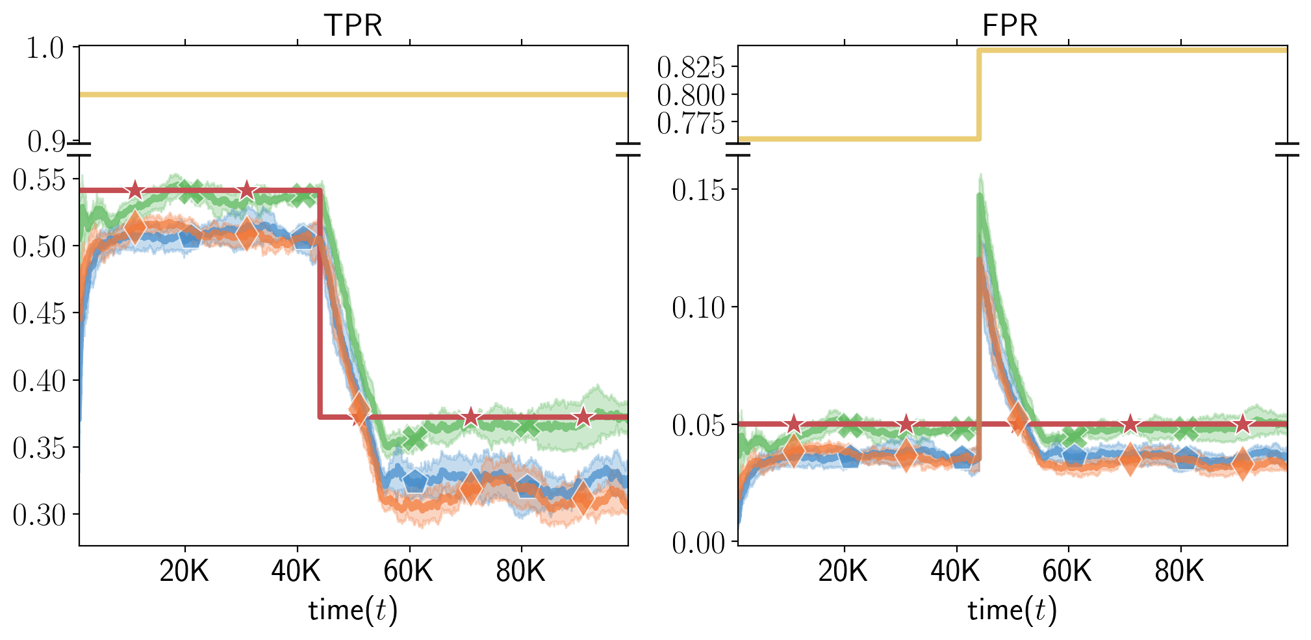}}
  }
  %\vspace{-5pt}
  \caption{\small{
    Results on the Virtual-logit Match (VIM) method with Cifar-10 as the ID dataset. }
    }
  \label{fig:vim-cifar10}
  \vspace{-5pt}
\end{figure*}
