# Supplementary material for: Taming False Positives in Out-of-Distribution Detection with Human Feedback
Source: arXiv:2404.16954 source file (2024-04-25)
Supplement: Supplementary file 14 [file sim_gamma_change.tex]

\begin{figure*}[t]
  \centering
  \includegraphics[width=0.999\textwidth]{figs/fprtpr8/legend.png}
  \mbox{
  \hspace{-10pt}
    \subfigure[No window, $\gamma$ changes suddenly.  \label{fig:sim_gamma_change_sudden}]{\includegraphics[scale=0.18]{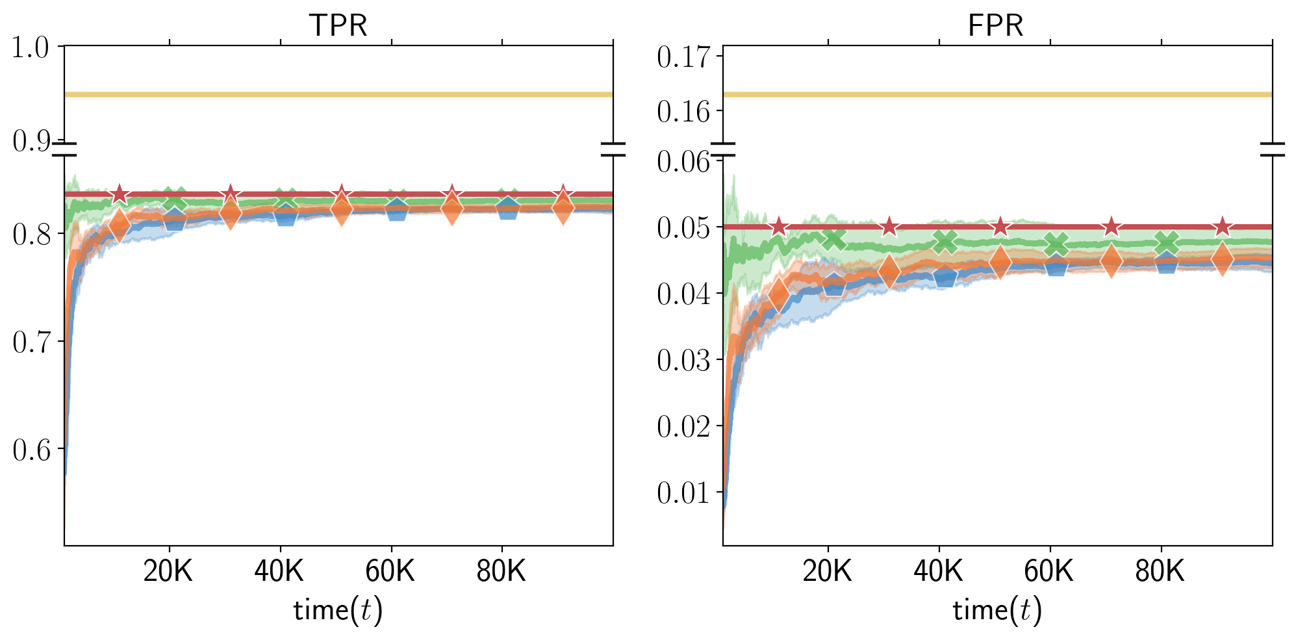}}
    \hspace{1pt}
    
    \subfigure[10k window, $\gamma$ changes suddenly. \label{fig:fig:sim_gamma_change_sudden_win_10k}]{\includegraphics[scale=0.18]{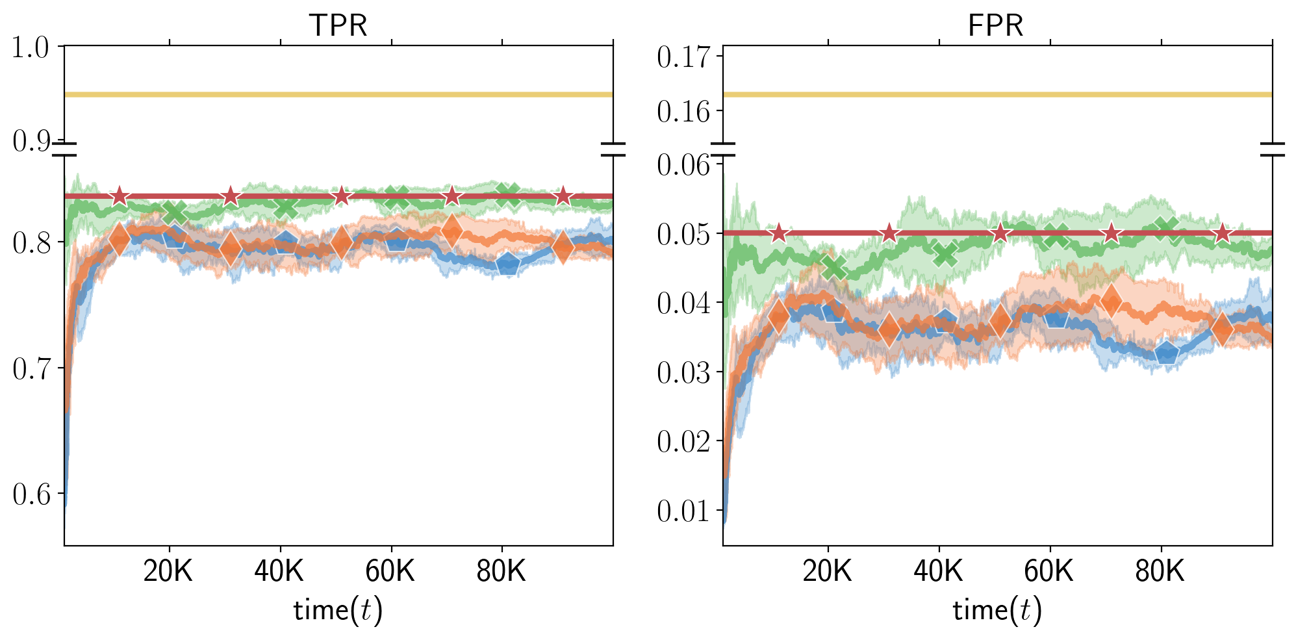}}
  }
  \mbox{
  %\hspace{-12pt}
    \subfigure[No window, $\gamma$ changes gradually. \label{fig:sim_gamma_change_gradual}]{\includegraphics[scale=0.18]{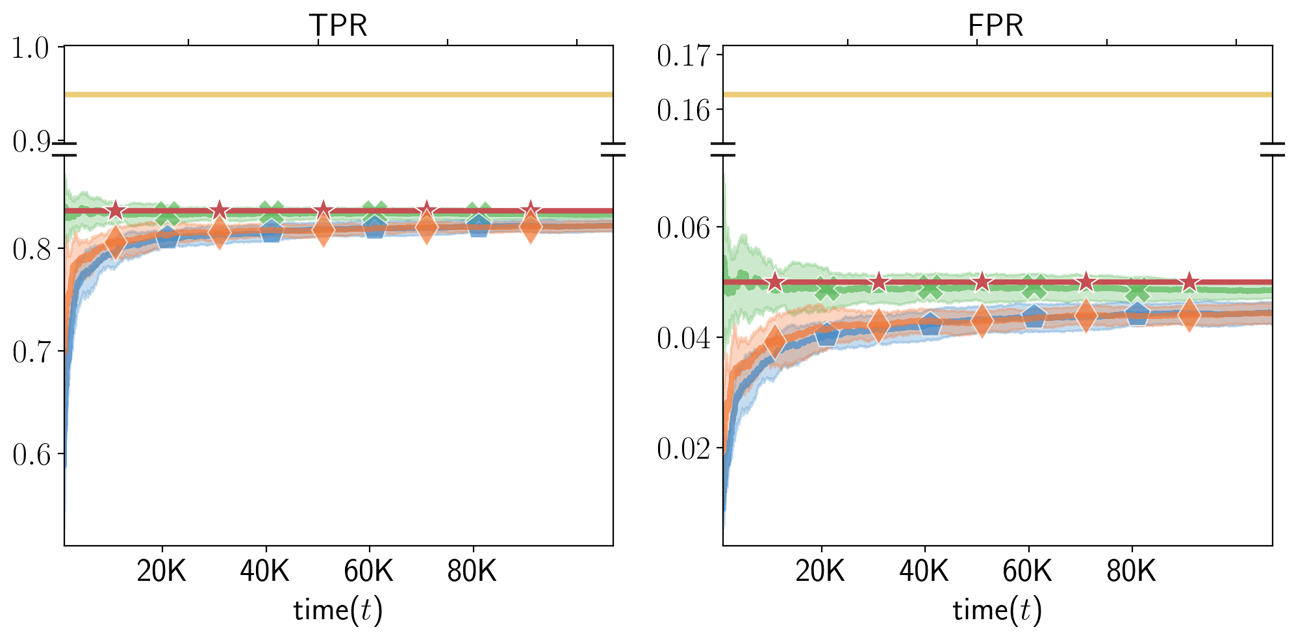}}
    %\hspace{1pt}
    
    \subfigure[10k window, $\gamma$ changes gradually.\label{fig:sim_gamma_change_gradual_win_10k}]{\includegraphics[scale=0.18]{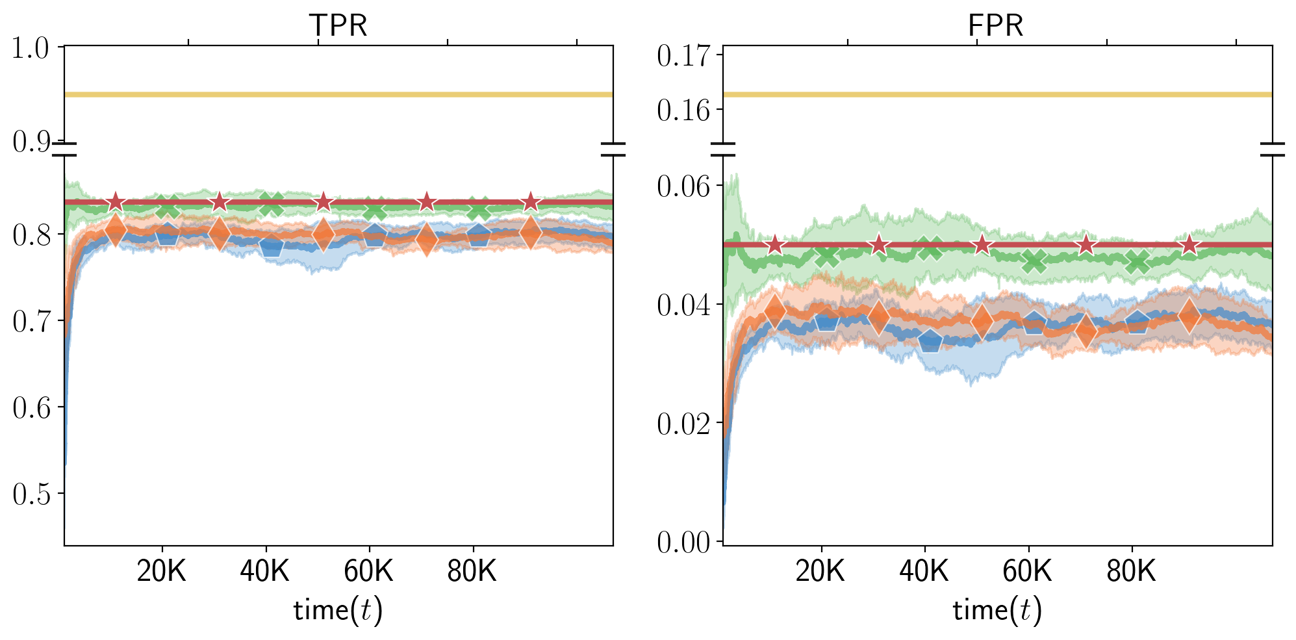}}
  }
  %\vspace{-5pt}
  \caption{
    Changing the mixing ratio $\gamma$ in the synthetic data. 
    }
  \label{fig:sim-gamma-change}
  
\end{figure*}
