# Supplementary material for: Taming False Positives in Out-of-Distribution Detection with Human Feedback
Source: arXiv:2404.16954 source file (2024-04-25)
Supplement: Supplementary file 15 [file sim_id_change.tex]

\begin{figure*}[t]
  %\vspace{-8pt}
  \centering
  \includegraphics[width=0.999\textwidth]{figs/fprtpr8/legend.png}
  \mbox{
  \hspace{-10pt}
    \subfigure[No window.  \label{fig:sim_id_shift_win_no}]{\includegraphics[scale=0.18]{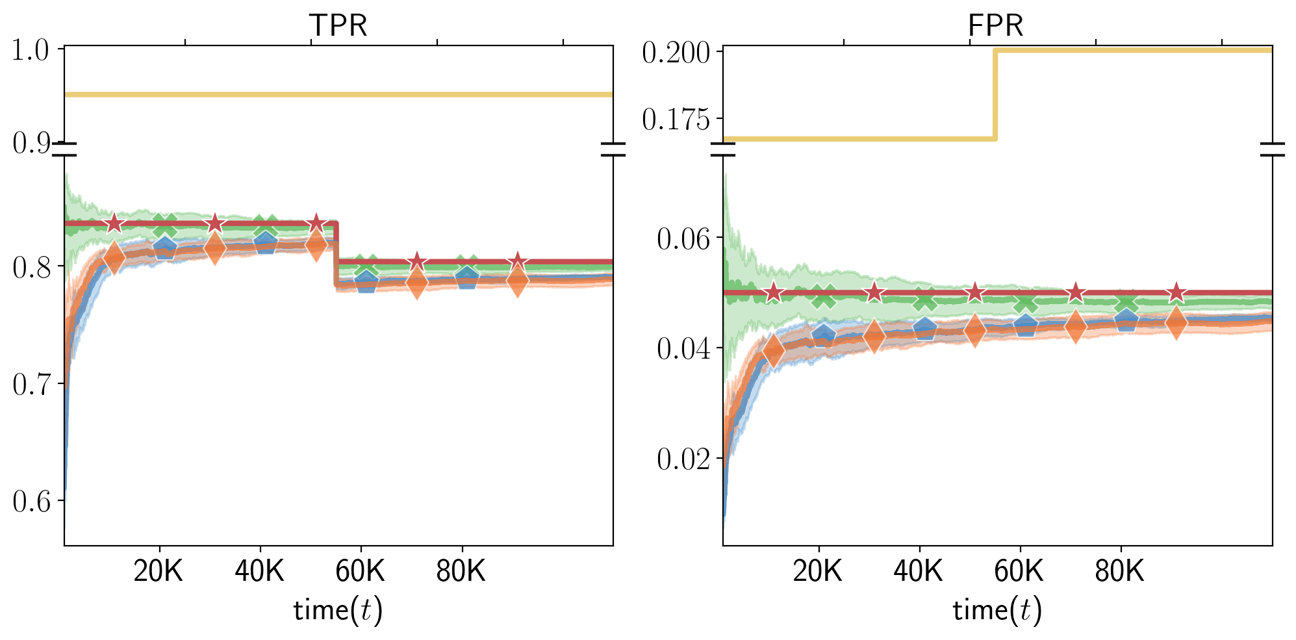}}
    \hspace{1pt}
    
    \subfigure[10k window. \label{fig:sim_id_shiftwin_10k}]{\includegraphics[scale=0.18]{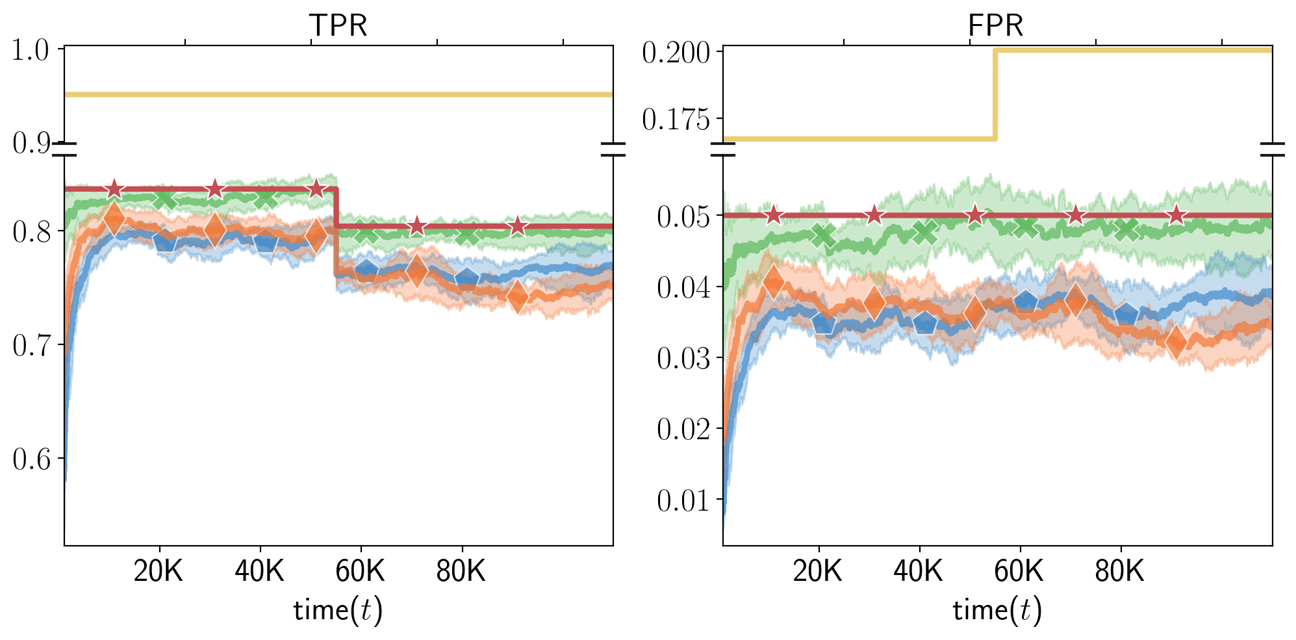}}
  }
  \caption{
    Changing ID distribution in synthetic data. 
    }
  \label{fig:sim-id-shift}
  %\vspace{-5pt}
\end{figure*}
