# Supplementary material for: Taming False Positives in Out-of-Distribution Detection with Human Feedback
Source: arXiv:2404.16954 source file (2024-04-25)
Supplement: Supplementary file 16 [file sim_no_change.tex]

\begin{figure*}[t]
  \centering
\includegraphics[width=0.999\textwidth]
  {figs/fprtpr8/legend.png}
  \centering
  \mbox{
  \hspace{-10pt}
    \subfigure[ No window, no distribution shift. \label{fig:sim_naive}]{\includegraphics[scale=0.32]{figs/newratio/sythetic/21_nowin.png}}
    \hspace{1pt}
    
    \subfigure[ 10K window, no distribution shift\label{fig:sim_win_10k}]{\includegraphics[scale=0.32]{figs/newratio/sythetic/21_10kwin.png}}
  }
  \mbox{
  \hspace{-10pt}
    \subfigure[ No window, distribution shift at $t=55k$. \label{fig:sim_shifted}]{\includegraphics[scale=0.32]{figs/newratio/sythetic/21_shifted_nowin.png}}
    \hspace{1pt}
    \subfigure[10K window, distribution shift at $t=55k$.\label{fig:sim_shifted_win_10k}]{\includegraphics[scale=0.33]{figs/newratio/sythetic/21_shifted_10kwin.png}}
  }
  %\vspace{-8pt}
  \caption{
    Experiments on Synthetic Data. The ratio of ID: OOD = 2:1. Each method is repeated 10 times. The mean and standard deviation are shown. The distribution shift starts at $t=55k$ for figure \ref{fig:sim_shifted},\ref{fig:sim_shifted_win_10k}. 
    }
  \label{fig:sim-no-change-21}
  %\vspace{-10pt}
\end{figure*}

\begin{figure*}[t]
  \centering
\includegraphics[width=0.999\textwidth]
  {figs/fprtpr8/legend.png}
  \centering
  \mbox{
  \hspace{-10pt}
    \subfigure[ No window, no distribution shift. \label{fig:sim_naive}]{\includegraphics[scale=0.32]{figs/newratio/sythetic/41_nowin.png}}
    \hspace{1pt}
    
    \subfigure[ 10K window, no distribution shift\label{fig:sim_win_10k}]{\includegraphics[scale=0.32]{figs/newratio/sythetic/41_10kwin.png}}
  }
  \mbox{
  \hspace{-10pt}
    \subfigure[ No window, distribution shift at $t=55k$. \label{fig:sim_shifted}]{\includegraphics[scale=0.32]{figs/newratio/sythetic/41_shifted_nowin.png}}
    \hspace{1pt}
    \subfigure[10K window, distribution shift at $t=55k$.\label{fig:sim_shifted_win_10k}]{\includegraphics[scale=0.33]{figs/newratio/sythetic/41_shifted_10kwin.png}}
  }
  %\vspace{-8pt}
  \caption{
    Experiments on Synthetic Data. The ratio of ID: OOD = 4:1. Each method is repeated 10 times. The mean and standard deviation are shown. The distribution shift starts at $t=55k$.
    }
    \label{fig:sim-no-change-41}
  %\vspace{-10pt}
\end{figure*}


%\begin{figure*}[t]
%  \centering
%\includegraphics[width=0.999\textwidth]
%  {figs/fprtpr8/legend.png}
%  \centering
%  \mbox{
%  \hspace{-10pt}
%    \subfigure[ No window, no distribution shift. \label{fig:sim_naive}]{\includegraphics[scale=0.32]{figs/fprtpr8/sim.png}}
%    \hspace{1pt}
%    
%    \subfigure[ 10K window, no distribution shift\label{fig:sim_win_10k}]{\includegraphics[scale=0.32]{figs/fprtpr8/sim_win_10k.png}}
%  }
%  \mbox{
%  \hspace{-10pt}
%    \subfigure[ No window, distribution shift at $t=55k$. \label{fig:sim_shifted}]{\includegraphics[scale=0.32]{figs/fprtpr8/sim_shifted.png}}
%    \hspace{1pt}
%    \subfigure[10K window, distribution shift at $t=55k$.\label{fig:sim_shifted_win_10k}]{\includegraphics[scale=0.33]{figs/fprtpr8/sim_shifted_win_10k.png}}
%  }
%  %\vspace{-8pt}
%  \caption{
%    Experiments on Synthetic Data. Each method is repeated 20 times. The mean and standard deviation is shown. The distribution shift starts at $t=55k$ for figure \ref{fig:sim_shifted},\ref{fig:sim_shifted_win_10k}.
%    }
%  \label{fig:sim-no-change}
%  %\vspace{-10pt}
%\end{figure*}
